# Supplementary material for: Adaptive Sampling for Estimating Multiple Probability Distributions
Source: arXiv:1910.12406 source file (2019-12-07)
Supplement: Supplementary file 1 [file appendix_Experiments.tex]

In Figure~\ref{fig:figure2} we show the variation of the approx-oracle allocation and the allocation of the proposed adaptive schemes for the three distance measures, $\ell_2^2$, $\ell_1$ and separation distance. As we can see, for these three distance measures, the adaptive allocation closely followed the approx-oracle allocation, and the deviation between the two schemes decreased with increasing $n$.

For the case of KL-divergence for this class of problems considered, we computed the approx-oracle allocation numerically by exhaustively searching and  selecting the pair $(\Tins[1], \Tins[2])$ which equalized or almost equalized~\eqref{eq:kl_objective}. As $\epsilon$ was varied in the set $\{0.05, \ldots, 0.95\}$ we found that the approx-oracle allocation was within a few samples  for all value of $n$ considered in the range $(100, 3000)$. This was also observed in adaptive allocation in the experiments.

\begin{figure*}[!h]
  \begin{subfigure}[t]{.5\textwidth}
    \centering
    \includegraphics[width=\linewidth, height=6cm]{allocation_200.pdf}
    % \caption{\textbf{Schnitt}: $A \cup B$: Element liegt in $A$ \textbf{oder} in $B$.}
  \end{subfigure}
  \hfill
  \begin{subfigure}[t]{.5\textwidth}
    \centering
    \includegraphics[width=\linewidth, height=6cm]{allocation_500.pdf}
    % \caption{ caption }
  \end{subfigure}

  \medskip
\vspace{-1em}
  \begin{subfigure}[t]{.5\textwidth}
    \centering
    \includegraphics[width=\linewidth, height=6cm]{allocation_1000.pdf}
    % \caption{caption }
  \end{subfigure}
  \hfill
  \begin{subfigure}[t]{.5\textwidth}
    \centering
    \includegraphics[width=\linewidth, height=6cm]{allocation_2000.pdf}
    % \caption{caption 4}
  \end{subfigure}
  
  \caption{The figures plots the number of samples allocated to the second arm (with distribution $P_\epsilon$) by the 
   Approx-Oracle allocation (AO) and the Adaptive allocation~(Ad) for $\ell_1$, $\ell_2$ and separation distance as the value of $\epsilon$ was varied from $0.1$ to $0.9$ for $L=10$ for $n \in \{200, 500, 1000, 2000\}$ }
  \label{fig:figure2}
\end{figure*}

We next have a table showing how the difference in the risk of the uniform allocation $\mc{A}_u$ and the adaptive allocation $\mc{A}$ varied for a fixed value of $n$ and changing values of $\epsilon$. From Fig.~\ref{fig:figure2}, we can see that for the $\ell_2$, $\ell_1$ and separation, with increasing value of $\epsilon$, the approx-optimal allocation $(\Tins)_{i=1}^2$ deviate further from the uniform allocation. This suggests that the gap in performance, in terms of the difference in risk or equivalently the difference in regret, should increase with $\epsilon$. 

\begin{table}[!h]
    \centering
   \begin{tabular}{c|rrrrrrrrr}
\hline
\backslashbox{$D$}{$\epsilon$}& $0.1$ & $0.2$ & $0.3$ & $0.4$ & $0.5$ & $0.6$ & $0.7$ & $0.8$ & $0.9$ \\ \hline 
$\ell_2$ & 0.0003 &  0.0004 &  0.0006 &  0.0007 & 0.0031 & 0.0028 & 0.0073 & 0.0125 &  0.0128 \\
$\ell_1$ &-0.0002 &  0.0032 &  0.0006 &  0.0075 & 0.0092 & 0.0146 & 0.0141 & 0.0234 &  0.0252 \\
KL  &0.0000 &  0.0006 &  0.0004 &  0.0003 & 0.0003 & 0.0003 & 0.0006 & 0.0002 &  0.0015 \\
 Sep. &0.0008 &  0.0111 &  0.0064 &  0.0267 & 0.0369 & 0.0521 & 0.0712 & 0.0943 &  0.1597 \\
\hline
\end{tabular}
    \caption{Table shows the values of the Difference of the estimated risk $(\mc{L}_n)$ of uniform and adaptive scheme (i.e., $\mc{L}_n \lp \mc{A}_u, \cdot\rp - \mc{L}_n \lp \mc{A}, \cdot\rp $) with $n$ fixed at $500$. The general trend for $\ell_2$, $\ell_1$ and separation is that as $\epsilon$ increases, the difference in performance between uniform and adaptive allocation also widens.}
    \label{tab:my_label}
\end{table}
